# Supplementary material for: FLARE: Agentic Coverage-Guided Fuzzing for LLM-Based Multi-Agent Systems
Source: arXiv:2604.05289 source file (2026-04-07)
Supplement: Supplementary file 1 [file 8.Appendix.tex]

\section{Appendix}\label{prompt-design}
% \begin{figure*}
%     \centering
%     \includegraphics[width=\textwidth]{image/Prompt.png}
%     \caption{Prompt Design of \tool.}
%     \label{prompt}
% \end{figure*} 
